# Supplementary material for: Open-Vocabulary SAM: Segment and Recognize Twenty-thousand Classes Interactively
Source: arXiv:2401.02955 source file (2024-09-14)
Supplement: Supplementary file 1 [file main_supp.tex]

\documentclass[runningheads]{llncs}

% ---------------------------------------------------------------
% Include basic ECCV package
 
% TODO REVIEW: Insert your submission number below by replacing '*****'
% TODO FINAL: Comment out the following line for the camera-ready version
% \usepackage[review,year=2024,ID=6014]{eccv}
% TODO FINAL: Un-comment the following line for the camera-ready version
\usepackage{eccv}

% OPTIONAL: Un-comment the following line for a version which is easier to read
% on small portrait-orientation screens (e.g., mobile phones, or beside other windows)
%\usepackage[mobile]{eccv}

% ---------------------------------------------------------------
% Other packages

% Commonly used abbreviations (\eg, \ie, \etc, \cf, \etal, etc.)
\usepackage{eccvabbrv}

% Include other packages here, before hyperref.
\usepackage{graphicx}
\usepackage{booktabs}

\usepackage{pifont}
% The "axessiblity" package can be found at: https://ctan.org/pkg/axessibility?lang=en
\usepackage[accsupp]{axessibility}  % Improves PDF readability for those with disabilities.
\usepackage[export]{adjustbox}

% ---------------------------------------------------------------
% Hyperref package

% It is strongly recommended to use hyperref, especially for the review version.
% Please disable hyperref *only* if you encounter grave issues.
% hyperref with option pagebackref eases the reviewers' job, but should be disabled for the final version.
%
% If you comment hyperref and then uncomment it, you should delete
% main.aux before re-running LaTeX.
% (Or just hit 'q' on the first LaTeX run, let it finish, and you
%  should be clear).

% TODO FINAL: Comment out the following line for the camera-ready version
% \usepackage[pagebackref,breaklinks,colorlinks,citecolor=eccvblue]{hyperref}
% TODO FINAL: Un-comment the following line for the camera-ready version
\usepackage{hyperref}

% Support for ORCID icon
\usepackage{orcidlink}

% Additional Packages
\usepackage{multirow}
\usepackage{tabularx}
\begin{document}

% ---------------------------------------------------------------
% TODO REVIEW: Replace with your title
\title{Supplementary for Open-Vocabulary SAM}

% TODO REVIEW: If the paper title is too long for the running head, you can set
% an abbreviated paper title here. If not, comment out.
% \titlerunning{Abbreviated paper title}

% TODO FINAL: Replace with your author list. 
% Include the authors' OCRID for the camera-ready version, if at all possible.
\author{Haobo Yuan\inst{1}
\orcidlink{0000-0001-9770-7720}
\and
Xiangtai Li\inst{1}
% {\textsuperscript{$\dagger$}}
\orcidlink{0000-0002-0550-8247}
\and
Chong Zhou\inst{1}
\orcidlink{0000-0002-9776-7739}
\and
Yining Li\inst{2}
\orcidlink{0000-0003-1753-0887}
\and
Kai Chen\inst{2}
\orcidlink{0000-0002-6820-2325}
\and
Chen Change Loy\inst{1}
\orcidlink{0000-0001-5345-1591}
}

% TODO FINAL: Replace with an abbreviated list of authors.
\authorrunning{H. Yuan et al.}
% First names are abbreviated in the running head.
% If there are more than two authors, 'et al.' is used.

% TODO FINAL: Replace with your institution list.
\institute{
{\small S-Lab, Nanyang Technological University \and Shanghai AI Laboratory}\\
}

\maketitle

% \begin{abstract}
% \input{latex/0_abstract}
% \keywords{Scene Understanding \and  Open-Vocabulary \and SAM}
% \end{abstract}

\newcommand{\cavan}[1]{{\color{blue}(cavan: {#1})}} % cavan's comments
\newcommand{\lxt}[1]{{\color{cyan}(xiangtai: {#1})}} % xiangtai's comments
\newcommand{\chong}[1]{{\color{magenta}(chong: {#1})}} % Chong's comments

\input{ECCV24/latex/6_supp}
% \clearpage  % TODO REVIEW/FINAL: This \clearpage needs to be removed from both review and camera-ready versions.

% ---- Bibliography ----
%
% BibTeX users should specify bibliography style 'splncs04'.
% References will then be sorted and formatted in the correct style.
%
\bibliographystyle{splncs04}
\bibliography{ref}
\end{document}
